# Supplementary material for: LATex: Leveraging Attribute-based Text Knowledge for Aerial-Ground Person Re-Identification
Source: arXiv:2503.23722 source file (2025-10-30)
Supplement: Supplementary file 1 [file ICML2025_ID3843_SUPP.pdf]

# Appendices

We organize the appendix as follows:

- **Appendix A :** Details of the idealized assumption shown in Section 3.2 of the main paper.
- **Appendix B :** Additional implementation details of the proposed model.
- **Appendix C :** Extended experimental results, including numerical results and visualizations.

## A. Idealized Assumption Details

As elaborated in Section 3.2, the primary goal of the idealized assumption is to validate the feasibility of utilizing person attribute information as auxiliary data for cross-view person retrieval, as well as to explore the theoretical upper bound under a CLIP-based prompt-tuning framework. The network archtecture of idealized assumption is shown in Fig. 9(a). For the input images $\mathcal{C}^{Img}$, we consider prompt-tuning CLIP visual encoder, which provides the visual features $F_v$. For the textual input, we encode the ground truth of person attributes into a predefined template, specifically, "A photo of a $Attribute$ person," to construct a contextualized text sequence. This sequence is then passed through the frozen CLIP text encoder to extract the corresponding textual feature $F_t$. $F_v$ and $F_t$ are supervised using the ReID loss defined in Eq. 11, respectively. During inference, the two features are concatenated as $[F_t, F_v]$ to form a unified feature vector for retrieval.

As shown in Fig. 9(b), under the same backbone configuration as our proposed LATex, the idealized assumption achieves near-perfect performance on the AG-ReID.v1 dataset. These remarkable idealized experimental results motivate us to explore more practical approaches aligned with real-world scenarios.

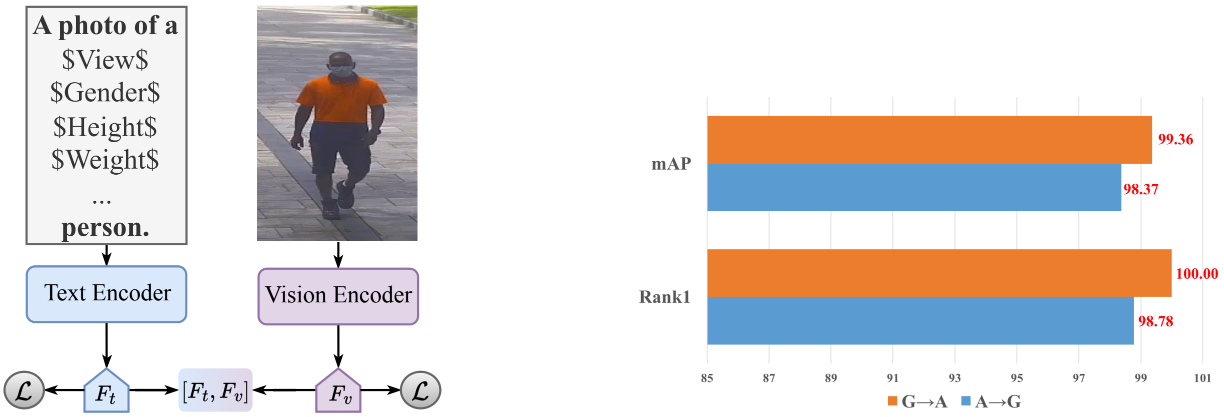


(a) Overview of idealized assumption

(b) Experiment results of idealized assumption

*Figure 9.* Overview and experiment results of idealized assumption.

## B. More Implementation Details

We provide more details information of experiment implementation in this section:

**LATex.** In addition to the implementation details described in the main text, we utilize the Adam optimizer with a base learning rate of 0.00035 and a weight decay of 0.1 to optimize our model. A learning rate scheduling strategy is employed, combining a warm-up phase with cosine decay and a scaling factor of 0.01. Finally, in the AIE module, we leverage a larger number of learnable prompts for large-scale datasets to achieve better performance. Specifically, we use 128 prompts for AG-ReID.v2 and 256 for CARGO. Notably, despite the increased number of learnable prompts, only the first $T$ prompts, corresponding to the total number of person attributes, are used as attribute-aware prompts in subsequent training as described in the main text. The remaining prompts are solely utilized for fine-tuning the pre-trained model.

**LATex†.** LATex† is a variant of LATex that adopts the full fine-tuning strategy to ensure a fair comparison with other AG-ReID methods employing the same training strategy. Specifically, we unfroze all trainable parameters of the pre-trained

*Table 8.* Performance comparison evaluated using the mINP metric. The superscript symbol † indicates results based on full fine-tuning strategies. The best and second-best results are highlighted in **bold** and <u>underline</u>.

| Method | AG-ReID.v1 | | CARGO | | | |
|---|---|---|---|---|---|---|
| | A→G | G→A | ALL | A↔G | G↔G | A↔A |
| ViT(Dosovitskiy et al., 2020) | - | - | 39.62 | 28.20 | 57.55 | 47.07 |
| VDT(Zhang et al., 2024b) | 51.06 | <u>52.87</u> | 41.13 | 29.95 | 58.39 | <u>50.22</u> |
| **LATex** | <u>51.28</u> | 50.95 | <u>44.24</u> | <u>36.64</u> | <u>62.53</u> | 39.28 |
| **LATex†** | **54.27** | **56.50** | **54.06** | **45.96** | **68.45** | **54.77** |

*Table 9.* Performance evaluated using the mINP metric. The superscript symbol † indicates results based on full fine-tuning strategies.

| Method | AG-ReID.v2 | | | |
|---|---|---|---|---|
| | A→C | A→W | C→A | W→A |
| **LATex** | 56.16 | 56.72 | 49.68 | 51.52 |
| **LATex†** | 63.43 | 61.87 | 55.84 | 56.74 |

CLIP vision and text encoders and updated them with a learning rate of 0.000005. Other experimental settings, including the learning rate decay strategy, optimizer, and the number of training epochs, are kept consistent with LATex.

**Idealized Assumption.** The idealized assumption represents a simplified version of LATex under ideal conditions, where only the backbone network of LATex is retained. All experimental settings are consistent with those of LATex.

# C. Extended Experiment

## C.1. More Performance Comparison

Tab. 8 compares the mINP performance of our model under various evaluation protocols on two AG-ReID benchmarks (AG-ReID.v1 and CARGO) with other Transformer-based methods. As the Explain (Nguyen et al., 2023b) neither reporte this metric in the paper nor release its code, we omit it from the table. For the same reason, Tab. 9 reports the mINP metric on AG-ReID.v2 exclusively for our proposed LATex and its variant LATex†. Consistent with the trends observed in the mAP and Rank-1 metrics discussed in the main text, LATex with a frozen backbone demonstrates superior aggregate performance. Meanwhile, with trainable backbone parameters, LATex† achieves the best results. Specifically, LATex† outperforms the previous best model, VDT, by over **13%** on average across all protocols on the CARGO benchmark.

## C.2. More Ablation Studies

Fig. 10 presents a more comprehensive ablation study on the effect of the number of learnable prompts on AG-ReID.v1 benchmark. Consistent with the conclusions we drawn in the main text, although slight fluctuations are observed, this factor is not a primary determinant of LATex's performance.

## C.3. More Visualization Analysis

Fig. 11 presents more detailed visualizations of retrieval results based on attribute features from query images. Despite challenges posed by complex visual conditions, LATex demonstrates robust fine-grained attribute perception performance.

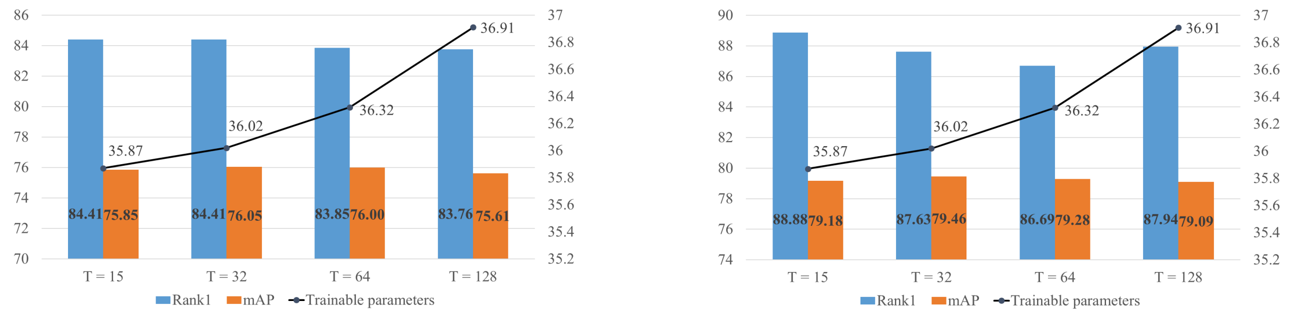


(a) A→G (b) G→A

*Figure 10.* Performance with different number of prompts on AG-ReID.v1.

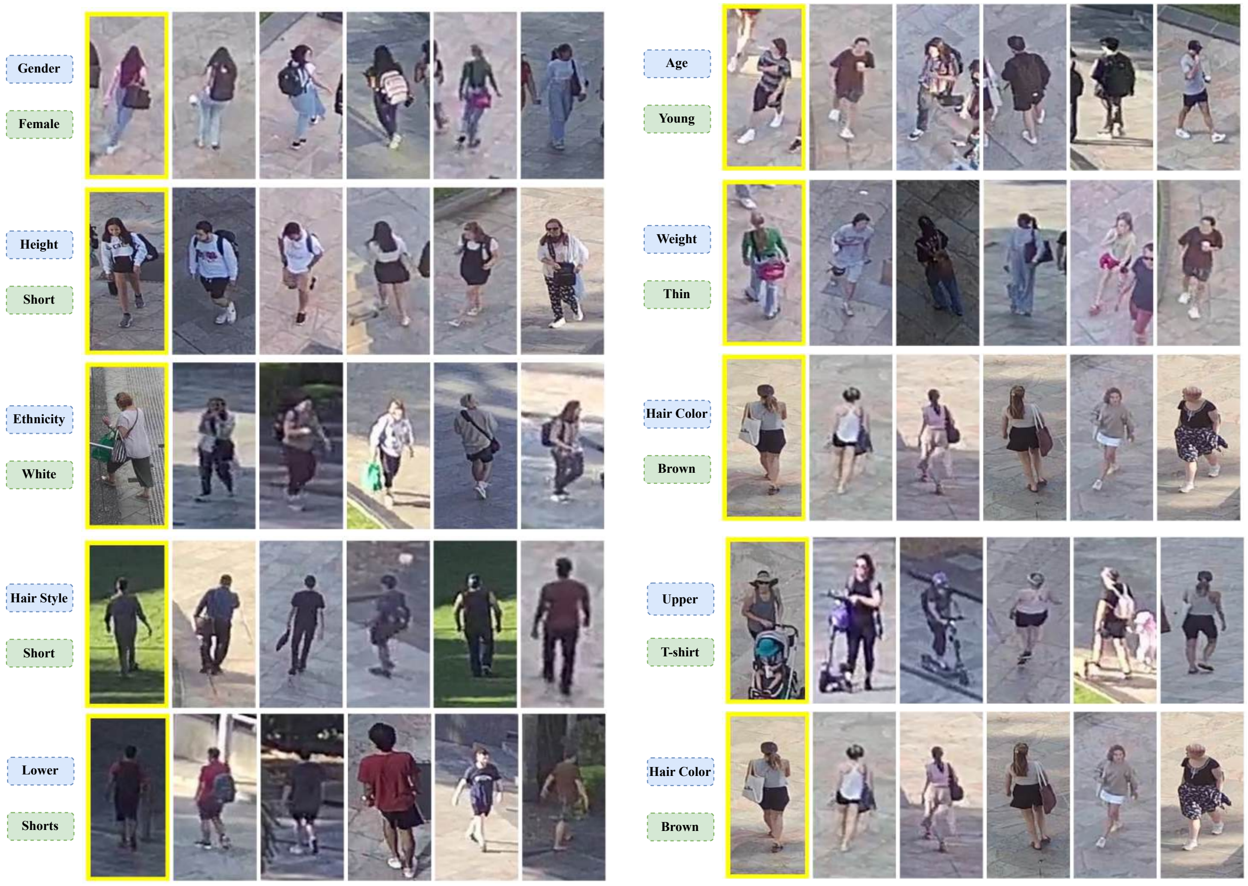


*Figure 11.* Visualizations of retrieval results based on attribute features. Query images are highlighted with yellow boxes, while the corresponding attribute names and ground truth values are displayed in blue and green boxes, respectively.
